# Supplementary material for: Hierarchical Interdisciplinary Topic Detection Model for Research Proposal Classification
Source: arXiv:2209.13519 source file (2023-02-22)
Supplement: Supplementary file 1 [file appendix.tex]

% For model implementation, we introduce the Transformer based model proposed in \cite{vaswani2017attention} and the Graph Convolution Network proposed in \cite{kipf2016semi}, which are both two state-of-the-art approaches and have demonstrated very competitive ability in combination with encoder-decoder based textual related models~\cite{devlin2018bert, vaswani2017attention} and structural related classification models~\cite{Chen2017, Anderson2018, peng2019hierarchical, zhou2020hierarchy}. 

\subsection{Graph Convolutional Networks} \label{appendix.gcn}
We adopt Graph Convolutional Networks (GCNs)~\cite{kipf2016semi} to extract the network-structured interdisciplinary knowledge from the Co-topic graph. 
GCN is the most popular and widely-used graph neural networks (GNNs), which is a deep graph information extractor that integrates node features and its local neighbors' information into low-dimensional representation vectors.

Formally, given a graph $G$, suppose $\mathcal{W}\in \mathbb{R}^{N \times N}$ is the adjacency matrix of graph topology, $\mathcal{H}^{0}\in \mathbb{R}^{N \times h}$ is the node feature matrix, $N$ is the total number of nodes, and $h$ is the dimension of node feature.
GCN uses an efficient layer-wise propagation rule based on a first-order approximation of spectral convolutions on graphs. 
The $l$-th GCN layer can be formulated as:

\begin{equation}
\begin{aligned}
    \mathcal{H}^{(l+1)} &= GCNlayer(\mathcal{W},\mathcal{H}^{(l)})\\
    &= \sigma(\tilde{\mathcal{W}}\mathcal{H}^{(l)}W^{(l)})
    %&X =H^{(0)}\\
    %&H^{(l+1)} = \sigma(\tilde{D}^{-\frac{1}{2}}\tilde{A}\tilde{D}^{-\frac{1}{2}}H^{(l)}W^{(l)})\\
    %&Z =H^{(L)}
\end{aligned}
\end{equation}
where $\mathcal{H}^{(l+1)}\in \mathbb{R}^{N \times h}$ is the output of the GCN layer, $W^{(l)}\in \mathbb{R}^{h \times h}$ is the layer-specific parameter matrix, $h$ is the hidden dimension, $\sigma$ denotes an activation function. $\tilde{\mathcal{W}}= \tilde{D}^{-\frac{1}{2}}\bar{\mathcal{W}}\tilde{D}^{-\frac{1}{2}}$, $\bar{\mathcal{W}} = A+I_N$, $I_N$ is the identity matrix and $\tilde{D}$ is the diagonal degree matrix of $\bar{\mathcal{W}}$.

In summary, after a $N$-layer GCN's propagation, formulated as $\mathcal{H}^{(N)} = N \times  GCNlayer(\mathcal{W},\mathcal{H}^{(0)})$, we can obtain the final node embedding matrix $\mathcal{H}^{(N)}\in \mathbb{R}^{N \times h}$, where each node embedding is integrated with the its $N$-hops neighborhood information.

\subsection{Transformer Details} \label{appendix.transformer}
A Transformer~\cite{vaswani2017attention} model usually has multiple layers. A layer of transformer model (i.e, a Transformer block) consists of a \textit{Multi-Head Self-Attention Layer}, a \textit{Residual Connections and Layer Normalization Layer}, a \textit{Feed Forward Layer}, and a \textit{Residual Connections and  Normalization Layer}, which can be written as:

\begin{equation}
\label{eq:3}
    Z^{(l)} = LN(X^{(l)}+MultiHead(X^{(l)},X^{(l)},X^{(l)})),
\end{equation}

\begin{equation}
\label{eq:4}
    X^{(l+1)} =  LN(Z^{(l)}+FC((Z^{(l)})),
\end{equation}

where $X^{(l)} = [x_1^{(l)}, x_2^{(l)}, ..., x_s^{(l)}]$ is the input sequence of $l$-th layer of Transformer, $s$ is the length of input sequence, $ x_i^{(l)}\in \mathbb{R}^h$ and $h$ in the dimension. $LN(\cdot)$ is layer normalization, $FC(\cdot)$ denotes a two-layer feed-forward network with $ReLU$ activation function, and $MultiHead(\cdot)$ denotes the multi-head attention layer, which is
calculated as follows:

\begin{equation}
\label{eq5}
MultiHead(Q, K, V) = Concat (head_1, . . . , head_h)W^O,
\end{equation}

\begin{equation}
head_i = Attention(Q W_i^Q,K W_i^K,V W_i^V),
\end{equation}

\begin{equation}
\label{eq7}
Attention (Q,K,V) = softmax(\frac{QK^T}{\sqrt{d}})V,
\end{equation}

where $W_i^Q, W_i^K, W_i^V\in \mathbb{R}^{h\times h}$ are weight matrices and $d$ is the number of attention heads. After the attention calculation, the $h$ outputs are concatenated and
transformed using a output weight matrix $W^O\in \mathbb{R}^{dh\times h}$.

In summary, given the input token sequence $X = [x_1, x_2, ..., x_s]$, we first initilize the input matrix  $X^{(0)} = [x_1^{(0)}, x_2^{(0)}, ..., x_s^{(0)}]$ before the first layer by a look-up table. Then, after the propagation in Equation \ref{eq:3} and \ref{eq:4} on a $N$-layers Transformer, formulized as $X^{(N)} = N \times Transformer(X^{(0)})$, we can obtain the final output embeddings of this sequence $X^{(N)} = [x_1^{(N)}, x_2^{(N)}, ..., x_s^{(N)}]$, where each embedding has contained the context information in this sequence.  The main hyper-parameters of a Transformer are the number of layers (i.e., Transformer blocks), the number of self-attention heads, and the maximum length of inputs.
